# Supplementary material for: Query Reranking As A Service
Source: arXiv:1602.05100 source file (2016-07-16)
Supplement: Supplementary file 1 [file appendix.tex]

\appendix

\section{MD Pseudocodes}
\vspace{2mm}

\vspace{2mm}
